# Supplementary material for: Sketch-Guided Constrained Decoding for Boosting Blackbox Large Language Models without Logit Access
Source: arXiv:2401.09967 source file (2024-07-22)
Supplement: Supplementary file 1 [file 04_IE_GCD_VS_AGCD.tex]

\section{GCD vs. AGCD for Closed IE}\label{app_sec:agcd_vs_gcd_cie}
xxx

\input{tables/appendix/IE_GCD_VS_AGCD_results}
