# Supplementary material for: Sketch-Guided Constrained Decoding for Boosting Blackbox Large Language Models without Logit Access
Source: arXiv:2401.09967 source file (2024-07-22)
Supplement: Supplementary file 2 [file CD.tex]

\section{Constrained Decoding}\label{sec:constraint-decoding-with-logits}

The decoding problem in natural language generation can be formulated as the search for the most likely sequence $y^*$ given a LM $q$ and an input sequence $x$:
\begin{equation*}
    y^* = \argmax_{y \in \mathcal{Y}} q(y|x)
\end{equation*}
where $\mathcal{Y}$ is the set of all possible output sequences.

Given the autoregressive nature of most LLMs, the conditional probability $q(y|x)$ can be decomposed into a product of conditional probabilities of each token $y_i$ given the prefix $y_{<i}$:
\begin{equation*}
    y^* = \argmax_{y \in \mathcal{Y}} \prod_{i=1}^{|y|} q(y_i|y_{<i}, x)
\end{equation*}

\textit{Constrained decoding} modifies the decoding problem by restricting the search space to a subset of $\mathcal{Y}$ that satisfies the constraints $\mathcal{C}$, \ie, $\mathcal{Y} \cap \mathcal{C}$.
Several frameworks have been proposed to systematically specify constraints $C$ for various tasks, including automaton-based constraints~\citep{deutsch-etal-2019-general}, grammar-based constraints~\citep{yin-neubig-2017-syntactic}, and energy function-based constraints~\citep{qin_cold_2022}.

Similarly to the free-text decoding problem, constrained decoding also faces the challenges of an exponentially large search space.
Constrained greedy search and constrained beam search~\citep{hokamp_lexically_2017} are two simple yet effective methods to approximately solve the constrained decoding problem.
Under the greedy search setting, each token $y_t$ is greedily selected to maximize the conditional probability $q(y_t|y_{<t}, x)$ at each step $t$ to ensure that the generated token $y_t$ satisfies the constraints $C$:
\begin{equation*}
    y_t^* = \argmax_{y_t \in \mathcal{Y}} q(y_t|y_{<t}, x) \cdot \mathbbm{1}(y_t \in C(y_{<t})),
\end{equation*}
in which $\mathbbm{1}(y_t \in C(y_{<t}))$ is 1 if $y_{\leq t}$ can lead to a valid output and 0 otherwise.

%TODO, the above usage of C is an abuse

The generation process terminates when the end-of-sequence token is generated.
The final output sequence $y^*$ is guaranteed to satisfy the constraints $C$.
